# Supplementary material for: Adversarial and Reactive Traffic Entities for Behavior-Realistic Driving Simulation: A Review
Source: arXiv:2409.14196 source file (2025-05-06)
Supplement: Supplementary file 1 [file 08_supplemental_material.tex]

\section{Comparison of Traffic Simulators}

\newpage
\section{Comparison of Trajectory Datasets}

\begin{table}[h!]
    \footnotesize
    \centering
    \caption{Comparison of recent trajectory datasets for road vehicles inspired by \cite{caesar_nuplan_2021, gressenbuch_mona_2022}. \textit{Record time}: Total duration of recorded trajectory data. \textit{Scenes}: Number of distinct locations. \textit{Sampling Frequency}: Frequency of trajectory positions. \textit{Sensor Data}: Availability of sensor data. \textit{Type}: Type of dataset, which can be either prediction ("Pred") or planning ("Plan").} 
    \begin{tabular}{lccccc}
        \toprule
        Dataset & \makecell{Record\\time} & \makecell{Scenes} & \makecell{Sampling \\ frequency} & \makecell{Sensor \\ data} & Type \\
        \midrule 

        CommonRoad \cite{althoff_commonroad_2017} & - & 39799 & 10 Hz & & Plan \\

        highD \cite{krajewski_highd_2018} & 16.5 h & 6 & 25 Hz & & Pred\\

        Argoverse 1 \cite{chang_argoverse_2019} & 320 h & 323,557 & 10 Hz & & Pred\\
        
        Interaction \cite{zhan_interaction_2019} & 10 h & 11 & 10 Hz & & Pred\\

        inD \cite{bock_ind_2020} & 10 h & 4 & 10 Hz & & Pred\\

        openDD \cite{breuer_opendd_2020}&  62 h & 7 & 10 Hz & & Pred\\

        nuPredict \cite{caesar_nuscenes_2020} \tablefootnote[1]{Human-labeled scenes from the nuScenes datase} & 5.5 h & 850 & 2 Hz & $\surd$ & Pred\\

        Waymo \cite{sun_scalability_2020} & 570 h & 103,354 & 10 Hz & &  Pred\\

        Lyft Level 5 \cite{houston_one_2021} & 1118 h & 170,000 & 10 Hz & & Pred\\

        Shifts \cite{malinin_shifts_2021} & 1667 h & - & 5 Hz & & Pred \\

        MONA \cite{gressenbuch_mona_2022} & 130 h & 3 & 5 Hz & & Pred \\ 

        Argoverse 2 \cite{wilson_argoverse_2023} & 763 h & 250,000 & 10 Hz& & Pred\\

        nuPlan \cite{caesar_nuplan_2021, karnchanachari_towards_2024} & 1282 h & - & 10 Hz & $\surd$ & Plan\\
        \bottomrule
    \end{tabular}
    \label{tab:datasets}
\end{table}

%\section{Definition of Evaluation Metrics} \label{sec:metrics_definitions}
%
%\subsection{Non-learned Evaluation Metrics}
%
%\textbf{Scene Average Displacement Error (SADE)}: 
%\begin{equation}
%\text{sADE} = \frac{1}{K_{te} N_I T} \sum_{k=1}^{K_{te}} \left[\sum_{i \in I} \sum_{t=1}^{T} \delta\left(s^{i}_{k,t}, s'^{i}_{k,t}\right)\right]
%\end{equation}
%where $I$ is the set of indices of the interactive agents, $s'^{i}_{k,t}$ and $s^{i}_{k,t}$ are the states of the $i^{th}$ interactive agents in the $k^{th}$ simulated and reference trajectories, respectively, and $\delta$ is a Euclidean distance function. \cite{igl_symphony_2022}

%\textbf{Minimum Scene Average Displacement Error (minSADE)}: 
%\begin{equation}
%\text{minSADE} = \frac{1}{K_{te} N_I T} \sum_{k=1}^{K_{te}} \min_{r' \in R_k} \left[ \sum_{i \in I} \sum_{t=1}^{T} \delta\left(s^{i}_{k,t}, s'^{i}_{k,t}\right) \right],
%\end{equation}
%when $m = 1$, minSADE reduces to SADE; when $m > 1$, minimising minSADE requires populating Rk with diverse but realistic trajectories. \cite{igl_symphony_2022}

%\textbf{Coverage (cov) and diversity (div)}: 
%\begin{equation}
%    \text{Diversity} = \frac{2}{n(n-1)} \sum_{i=1}^{n-1} \sum_{j=i+1}^{n} \text{Wass}(\rho_i,\rho_j),
%\end{equation}
%where $\text{Wass}(\cdot,\cdot)$ is the Wasserstein distance and $\rho_i$ is the density profile for the $i$-th trail.

%\subsection{Learned Evaluation Metrics}
